# Supplementary material for: Bayesian model selection for exponential random graph models via adjusted pseudolikelihoods
Source: arXiv:1706.06344 source file (2017-10-19)
Supplement: Supplementary file 1 [file Supplementary_material.pdf]

# Supplementary material to "Bayesian model selection for exponential random graph models via adjusted pseudolikelihoods"

Lampros Bouranis, Nial Friel, Florian Maire
School of Mathematics and Statistics & Insight Centre for Data Analytics,
University College Dublin, Ireland

## 1 Methods to compute the model evidence

### 1.1 Chib and Jeliazkov's method

A popular method of marginal likelihood estimation within each model is that of Chib (1995). Following from Bayes' formula, the model evidence is given by the *basic marginal likelihood identity*

$$\pi(y) = \frac{f(y \mid \theta)p(\theta)}{\pi(\theta \mid y)}. \tag{S.1}$$

An estimate of the marginal likelihood $\log \pi(y) = \log f(y \mid \theta^\dagger) + \log p(\theta^\dagger) - \log \pi(\theta^\dagger \mid y)$ is obtained by evaluating this expression on the log scale at some specific point $\theta^\dagger \in \Theta$. By approximating the true likelihood with the adjusted pseudolikelihood and $\pi(\theta \mid y)$ with $\widetilde{\pi}(\theta \mid y)$, the first two terms are available by direct calculation. However, an estimate of the posterior ordinate $\widetilde{\pi}(\theta^\dagger \mid y)$ is still required. For estimation efficiency, the point $\theta^\dagger$ is chosen in a high density region of the support $\Theta$.

An extension of this work is provided in Chib and Jeliazkov (2001), where output from a Metropolis-Hastings algorithm for the posterior $\widetilde{\pi}(\theta \mid y)$ can be used to estimate the model evidence. Among others, the authors suggested the *one-block Metropolis-Hastings* approach for estimating the evidence, in the case where the parameter vector $\theta$ can be updated in a single block. For a Metropolis-Hastings transition from $\theta$ to $\theta'$, let $h(\theta, \theta')$ denote the candidate generating density and $\widetilde{\alpha}(\theta, \theta')$ denote the probability of accepting the proposed move when the corresponding Markov chain has $\widetilde{\pi}(\theta \mid y)$ as the limiting distribution. The proposed estimate of the posterior ordinate at $\theta^\dagger$ is

$$\hat{\widetilde{\pi}}(\theta^\dagger \mid y) = \frac{M^{-1}\sum_{m=1}^{M} \widetilde{\alpha}(\theta^{(m)}, \theta^\dagger) h(\theta^{(m)}, \theta^\dagger)}{L^{-1}\sum_{l=1}^{L} \widetilde{\alpha}(\theta^\dagger, \theta^{(l)})},$$

where $\{\theta^{(m)}\}$ are the sampled draws from the (corrected) pseudo-posterior and $\{\theta^{(l)}\}$ are the draws from $h(\theta^\dagger, \theta)$ given the fixed point $\theta^\dagger$. This gives

$$\log \widetilde{\pi}(y) = \log \tilde{f}(y \mid \theta^\dagger) + \log p(\theta^\dagger) - \log \hat{\widetilde{\pi}}(\theta^\dagger \mid y).$$

Chib and Jeliazkov (2001) generalised the method to settings with high-dimensional parameter spaces, which may require sampling of the parameters in several smaller blocks, eg. with a Metropolis-within-Gibbs strategy.

## 1.2 Power posteriors

Friel and Pettitt (2008) and Friel et al. (2014) demonstrated how the marginal likelihood can be computed via Markov chain Monte Carlo methods on modified posterior distributions for each model with the method of thermodynamic integration. They denote the power posterior by

$$\pi_t(\theta \mid y) \propto f(y \mid \theta)^t p(\theta),\ t \in [0,1],$$

where $z(y \mid t) = \int_\theta f(y \mid \theta)^t p(\theta)\, d\theta$ is the corresponding normalising constant.

The inverse temperature $t \in [0,1]$ has the effect of tempering the likelihood; at the extreme ends of the inverse temperature range, $\pi_{t=0}(\theta \mid y)$ and $\pi_{t=1}(\theta \mid y)$ correspond to the prior and posterior, respectively. Here we assume a prior distribution that leads to a finite $z(y \mid t)$ for all $t \in [0,1]$. When working with the corrected pseudo-posterior distribution, the respective version of the power posterior is:

$$\widetilde{\pi}_t(\theta \mid y) \propto \tilde{f}(y \mid \theta)^t p(\theta), \quad t \in [0,1], \tag{S.2}$$

The normalising constant is then expressed by

$$z(y \mid t) = \int_\Theta \tilde{f}(y \mid \theta)^t p(\theta)\, d\theta.$$

At zero temperature the integration is over the prior with respect to $\theta$, thus $z(y \mid t = 0) = 1$. We note that

$$\frac{d}{dt} \log z(y \mid t) = \mathbb{E}_{\theta|y,t} \log \tilde{f}(y \mid \theta),$$

therefore the log-evidence will be given by:

$$[\log z(y \mid t)]_0^1 = \log z(y \mid t = 1) = \int_0^1 \mathbb{E}_{\theta|y,t} \log \tilde{f}(y \mid \theta)\, dt. \tag{S.3}$$

To form an estimator based on (S.3) the inverse temperature range $t \in [0,1]$ is discretised as $0 = t_0 < t_1 < \ldots < t_m = 1$. A trapezoidal rule can be used to approximate the log-evidence:

$$\log \widetilde{\pi}(y) = \sum_{j=1}^{m} (t_j - t_{j-1}) \left[ \frac{\mathbb{E}_{\theta|y,t_{j-1}} \log \tilde{f}(y \mid \theta) + \mathbb{E}_{\theta|y,t_j} \log \tilde{f}(y \mid \theta)}{2} \right].$$

For each $t_j$, a MCMC sample from the posterior $\widetilde{\pi}_{t_j}(\theta \mid y)$ can be used to estimate $\mathbb{E}_{\theta|y,t_j} \log \tilde{f}(y \mid \theta)$, using a burn-in phase of $B < N$ iterations:

$$\mathbb{E}_{\theta|y,t_j} \log \tilde{f}(y \mid \theta) \approx \frac{1}{N - B} \sum_{i=B+1}^{N} \log \tilde{f}(y \mid \theta_j^{(i)}).$$

Three sources of error are present: error from discretisation of the temperature scheme, Monte Carlo error from approximating $\mathbb{E}_{\theta|y,t_j} \log \tilde{f}(y \mid \theta)$ and error coming from using the corrected pseudo-posterior. Estimating the marginal likelihood via the power posterior approach is rela-

tively straight-forward but computationally costly. To minimise the cost, it is desirable to use as few $t$ values as possible. However, choosing the temperature schedule presents an immediate difficulty with this approach.

A revised scheme by Friel et al. (2014) used an improved trapezoidal scheme for a more accurate quadrature approximation, which also requires the variance of the log likelihood. The authors proposed reducing the bias in the estimation of the marginal likelihood by observing that differentiation of $\mathbb{E}_{\theta|y,t} \log \tilde{f}(y \mid \theta)$ with respect to $t$ yields $\frac{d}{dt}\mathbb{E}_{\theta|y,t} \log \tilde{f}(y \mid \theta) = \mathbb{V}_{\theta|y,t} \log \tilde{f}(y \mid \theta)$. They improved upon the standard trapezoidal rule used to numerically integrate the expected log deviance by incorporating this derivative information at a minimal extra computational cost, yielding

$$\log \widetilde{\pi}(y) = \sum_{j=1}^{m} (t_j - t_{j-1}) \left[ \frac{\mathbb{E}_{\theta|y,t_{j-1}} \log \tilde{f}(y \mid \theta) + \mathbb{E}_{\theta|y,t_j} \log \tilde{f}(y \mid \theta)}{2} \right] - \frac{(t_j - t_{j-1})^2}{12} \left[ \mathbb{V}_{\theta|y,t_{j-1}} \log \tilde{f}(y \mid \theta) - \mathbb{V}_{\theta|y,t_j} \log \tilde{f}(y \mid \theta) \right], \quad \text{(S.4)}$$

having replaced the true likelihood with the pseudolikelihood approximation. The results presented in Section 7 are based on this improved trapezoidal scheme.

## 1.3 Applying control variates to evidence estimation

A key concern about the thermodynamic integral is that the corresponding evidence estimator can suffer from high variability. Oates et al. (2016) extended the zero-variance (ZV) control variate technique (Assaraf and Caffarel, 1999; Mira et al., 2013), aiming to improve the estimator by decreasing the variance. Together with the numerical integration scheme (S.4), the authors have shown that this can yield a dramatic improvement in the statistical efficiency of the estimate of the evidence by efficiently estimating $\mathbb{E}_{\theta|y,t_j} \log \tilde{f}(y \mid \theta)$ and $\mathbb{V}_{\theta|y,t_j} \log \tilde{f}(y \mid \theta)$ for each temperature $t_j \in [0,1]$, at very little extra computational cost.

The basic idea behind the control variate technique is to estimate the posterior expectation $\mathbb{E}_{\theta|y}[k(\theta)]$ by constructing a modified function $\tilde{k}(\theta) = k(\theta) + \phi_1 h_1(\theta) + \ldots + \phi_m h_m(\theta)$ such that $\tilde{k}(\theta)$ has the same posterior expectation but reduced posterior variance, compared to $k(\theta)$. This requires that each of the "control variates" $h_j(\theta)$ have zero posterior expectation, the collection $[h_1(\theta), \ldots, h_m(\theta)]$ has strong posterior canonical correlation with the target function $k(\theta) = \log \tilde{f}(y \mid \theta)$, and the coefficients $\phi_1, \ldots, \phi_m$ are appropriately selected.

Mira et al. (2013) and Oates et al. (2016) considered the class of control variates that are expressed as functions of the score vector $u(\theta \mid y)$ of the target function. By taking the target density to be the power posterior $\widetilde{\pi}_t(\theta \mid y)$, the score vector will be

$$u(\theta \mid y,t) = \nabla_\theta \log \widetilde{\pi}_t(\theta \mid y) = t \cdot \nabla_\theta \log \tilde{f}(y \mid \theta) + \nabla_\theta \log p(\theta).$$

Following Oates et al. (2016), the ZV control variates are

$$h(\theta \mid y,t) = \Delta_\theta[P(\theta \mid \phi(y,t))] + \nabla_\theta[P(\theta \mid \phi(y,t))] \cdot u(\theta \mid y,t),$$

where $\Delta_\theta = \nabla_\theta \cdot \nabla_\theta$ is the Laplacian operator and the "trial function" $P(\cdot)$ belongs to the family $\mathcal{P}$ of polynomials in $\theta$. The coefficients $\phi \equiv \phi(y,t)$ of the polynomial $P$ depend on both the data $y$ and inverse temperature $t$. This framework is highly compatible with the adjustment strategy

proposed in this paper; the replacement of the true (intractable) likelihood by the tractable likelihood approximation allows for ZV control variates that are in closed form. The "controlled thermodynamic integral" (CTI) will be

$$\log \widetilde{\pi}(y) = \int_0^1 \mathbb{E}_{\theta|y,t}\left[\log \tilde{f}(y \mid \theta) + h(\theta \mid y,t)\right] \, dt.$$

In this work we restrict our attention to degree 2 (quadratic) polynomials. Denoting the model dimensions by $d$, second degree polynomials can be expressed as $P(\theta) = c^T\theta + \frac{1}{2}\theta^T B\theta$ where $c$ is $d \times 1$ and $B$ is $d \times d$. This leads to ZV control variates of the form

$$h(\theta \mid y,t) = \mathrm{tr}(B) + (c + B\theta)^T u(\theta \mid y,t),$$

where $c$ and $B$ denote the quadratic polynomial coefficients and $\mathrm{tr}(B)$ is the trace of $B$. It is assumed that $B$ is symmetric, but this is not required in general. See Oates et al. (2016) for a further discussion of the ZV strategy with degree 2 polynomials.

Estimation of the control variates is performed with the same MCMC samples that are exploited to estimate $\mathbb{E}_{\theta|y,t} \log \tilde{f}(y \mid \theta)$ and $\mathbb{V}_{\theta|y,t} \log \tilde{f}(y \mid \theta)$. The control variates are stored along each Markov chain and their sample covariance is computed after the MCMC has terminated, leading to only a negligible increase in the total computational cost.

The optimal choice of polynomial coefficients, $\phi^*(y,t)$, that minimises the variance of the estimator of model log-evidence is given by

$$\phi^*(y,t) \approx -\hat{\mathbb{V}}^{-1}_{\theta|y,t}\left[u(\theta \mid y,t)\right] \hat{\mathbb{C}}_{\theta|y,t}\left[\log \tilde{f}(y \mid \theta), u(\theta \mid y,t)\right],$$

where $\hat{\mathbb{V}}_{\theta|y,t}\left[u(\theta \mid y,t)\right]$ and $\hat{\mathbb{C}}_{\theta|y,t}\left[\log f_{\mathrm{PL}}(y \mid g(\theta)), u(\theta \mid y,t)\right]$ denote the estimated variance and cross-covariance matrices, respectively.

To implement the second order quadrature rule proposed by Friel et al. (2014) we used the identity

$$\begin{aligned} \mathbb{V}_{\theta|y,t}\left[\log \tilde{f}(y \mid \theta) + h(\theta \mid y,t)\right] = {} & \mathbb{V}_{\theta|y,t}[\log \tilde{f}(y \mid \theta)] + \mathbb{V}_{\theta|y,t}[h(\theta \mid y,t)] \\ & + 2\mathbb{C}_{\theta|y,t}[\log \tilde{f}(y \mid \theta), h(\theta \mid y,t)]. \end{aligned}$$

If $\log \tilde{f}(y \mid \theta)$ and $h(\theta \mid y,t)$ are strongly correlated, so that the covariance term on the right hand side is greater than the variance of $h(\theta \mid y,t)$, then a variance improvement has been made over the original estimation problem.

Recently, Oates et al. (2017) generalised CTI beyond polynomials to general functions in a Hilbert space using a non-parametric extension of control variates. This methodology can possibly offer a route to further variance reduction.

## 1.4 The Stepping stones sampler

The Stepping stones sampler (Xie et al., 2011) uses the idea of powered posteriors (S.2), treating them as a series of intermediate distributions between the prior and the posterior. Based on importance sampling, the intermediate distributions are utilised as importance distributions, avoiding numerical integration. Following the notation of Friel et al. (2014), the method generates samples from each of the power posteriors from $t_0 = 0$ up to $t_{m-1}$, estimating the ratio of

consecutive normalising constants

$$r_k = \frac{z(y \mid t_{k+1})}{z(y \mid t_k)} = \int_\Theta \tilde{f}(y \mid \theta)^{t_{k+1}-t_k} \widetilde{\pi}_t(\theta \mid y)\, d\theta$$

with

$$\hat{r}_k = \frac{1}{N-B} \sum_{i=B+1}^{N} \tilde{f}(y \mid \theta^{(i)})^{t_{k+1}-t_k},\ k = 0, \ldots, m-1.$$

Here $N - B$ denotes the number of MCMC samples post burn-in and the corresponding sampled values $\{\theta^{(i)}\}$ are drawn from $\widetilde{\pi}_{t_k}$. Assuming that the prior is normalised, the final estimate of the model evidence will the product of these $m$ independent estimates, $\prod_{k=0}^{m-1} \hat{r}_k$, or at the log-scale:

$$\log \widetilde{\pi}(y) = \sum_{k=0}^{m-1} \log \hat{r}_k.$$

The Stepping stones estimator is unbiased for estimation of the marginal likelihood and biased for estimation of the log marginal likelihood. Xie et al. (2011) compared the performance of the Stepping stones sampler to that of power posteriors for estimating the log evidence. Their findings indicated that the Stepping stones approach slightly outperformed the power posterior, but the two approaches were comparable when the inverse temperature allocation was well chosen or when the number of inverse temperatures was large. The power posterior estimates performed relatively poorly when few inverse temperatures were present or when they were badly placed.

We observed the same comparable behaviour in our experiments, for a large number of rungs in the temperature ladder. Since the computational burden is mostly due to the simulation of the tempered distributions, one can easily calculate both estimates.

## 1.5 Population exchange algorithm

A population-based MCMC extension of the exchange algorithm (Møller et al., 2006), leading to realisations from the posterior distribution $\pi(\theta \mid y)$, was presented by Friel (2013). The algorithm was modified to allow for an unbiased estimate of the normalising constant of the likelihood, $z(\theta)$, for each draw $\theta$ from the posterior distribution.

The idea behind the method is to augment the target distribution with a sequence of tempered distributions by slowly moving from the prior, $\pi_{t_0}$, to the posterior, $\pi_{t_n}$. The augmented target distribution is

$$\pi_{t_0}(\theta_0 \mid y) \times \ldots \times \pi_{t_n}(\theta_n \mid y),\ \ t \in [0, 1],$$

where

$$\pi_{t_j}(\theta_j \mid y) \propto f(y \mid \theta_j)^{t_j} p(\theta_j).$$

The distribution of each chain in the population was further augmented in order to tackle the problem of likelihood intractability, yielding

$$\pi_{t_0}(\theta_0, \theta'_0, y'_{01}, \ldots, y'_{0s} \mid y) \times \ldots \times \pi_{t_n}(\theta_n, \theta'_n, y'_{n1}, \ldots, y'_{ns} \mid y),$$

where $\theta'_j$ is the auxiliary parameter value for the swap/exchange move and $y'_{j1}, \ldots, y'_{js} \sim f(y \mid \theta'_j)^{t_j}$ are draws from the tempered likelihood. At iteration $i$ of the Markov chain, those auxiliary

draws are used to estimate the normalising constant by

$$\hat{z}(\theta_n^{(i)}) = \prod_{j=0}^{n-1} \left( \frac{1}{s} \sum_{k=1}^{s} \frac{q(y_{jk}^{(i)'} \mid t_{j+1}\theta_{j+1}^{(i)})}{q(y_{jk}^{(i)'} \mid t_j \theta_j^{(i)})} \right) \times z(0).$$

The algorithmic output includes draws $\{\theta_n^{(i)}\}$ from the posterior distribution and associated estimates $\{\hat{z}(\theta_n^{(i)})\}$, which are used to approximate the marginal likelihood (S.1). Friel (2013) estimates the model evidence by

$$\hat{\pi}(y) := \frac{1}{r} \sum_{b=1}^{r} \hat{\pi}_{\theta_b}(y), \text{ where } \hat{\pi}_{\theta_b}(y) = \frac{q(y \mid \theta_b)}{\hat{z}(\theta_b)} \frac{p(\theta_b)}{\hat{\pi}(\theta_b \mid y)}, \tag{S.5}$$

for a range of draws $\{\theta_n^{(r)}\}_{r=1}^{b}$ from the high posterior density region, which requires kernel density estimation to estimate $\hat{\pi}(\theta_b \mid y)$.

# References


Assaraf, R. and M. Caffarel (1999). Zero-Variance principle for Monte Carlo algorithms. *Physical Review 83*(23), 4682–4685.

Chib, S. (1995). Marginal likelihood from the Gibbs output. *Journal of the American Statistical Association 90*(432), 1313–1321.

Chib, S. and I. Jeliazkov (2001). Marginal likelihood from the Metropolis-Hastings output. *Journal of the American Statistical Association 96*, 270–281.

Friel, N. (2013). Evidence and Bayes factor estimation for Gibbs random fields. *Journal of Computational and Graphical Statistics 22*(3), 518–532.

Friel, N., M. Hurn, and J. Wyse (2014). Improving power posterior estimation of statistical evidence. *Statistics and Computing 24*, 709–723.

Friel, N. and A. N. Pettitt (2008). Marginal likelihood estimation via power posteriors. *Journal of the Royal Statistical Society, Series B 70*(3), 589–607.

Mira, A., R. Solgi, and D. Imparato (2013). Zero Variance Markov chain Monte Carlo for Bayesian estimators. *Statistics and Computing 23*(5), 653–662.

Møller, J., A. Pettit, R. Reeves, and K. Bertheksen (2006). An efficient Markov chain Monte Carlo method for distributions with intractable normalising constants. *Biometrika 93*, 451–458.

Oates, C., M. Girolami, and N. Chopin (2017). Control functionals for Monte Carlo integration. *Journal of the Royal Statistical Society: Series B 79*(3), 695–718.

Oates, C., T. Papamarkou, and M. Girolami (2016). The controlled thermodynamic integral for Bayesian model evidence evaluation. *Journal of the American Statistical Association 111*(514), 634–645.

Xie, W., P. O. Lewis, Y. Fan, L. Kuo, and M. Chen (2011). Improving marginal likelihood estimation for Bayesian phylogenetic model selection. *Systematic Biology 60*(2), 150–160.
